# Supplementary material for: Bloch equations in Terahertz magnetic-resonance ellipsometry
Source: arXiv:2404.12805 source file (2024-04-19)
Supplement: Supplementary file 1 [file PRB_Supplementary.pdf]

# Supplementary material to: Bloch equations in Terahertz magnetic-resonance ellipsometry

Viktor Rindert,[1,2,3,*] Steffen Richter,[1,2] Philipp Kühne,[4,5,6] Alexander Ruder,[7] Vanya Darakchieva,[1,2,3,4] and Mathias Schubert[1,2,7]

[1]*NanoLund and Solid State Physics, Lund University, S-22100 Lund, Sweden*
[2]*Terahertz Materials Analysis Center, THeMAC, Lund University, S-22100 Lund, Sweden*
[3]*Center for III-Nitride Technology, C3NiT - Janzén, Lund University, S-22100 Lund, Sweden*
[4]*Department of Physics, Chemistry, and Biology (IFM), Linköping University, SE 58183, Linköping, Sweden*
[5]*Terahertz Materials Analysis Center, THeMAC, Linköping University, SE 58183, Linköping, Sweden*
[6]*Center for III-Nitride Technology, C3NiT - Janzén, Linköping University, SE 58183, Linköping, Sweden*
[7]*Department of Electrical and Computer Engineering, University of Nebraska-Lincoln, Lincoln, NE 68588, USA*
(Dated: April 19, 2024)

## I. FULL MUELLER MATRIX RESULTS

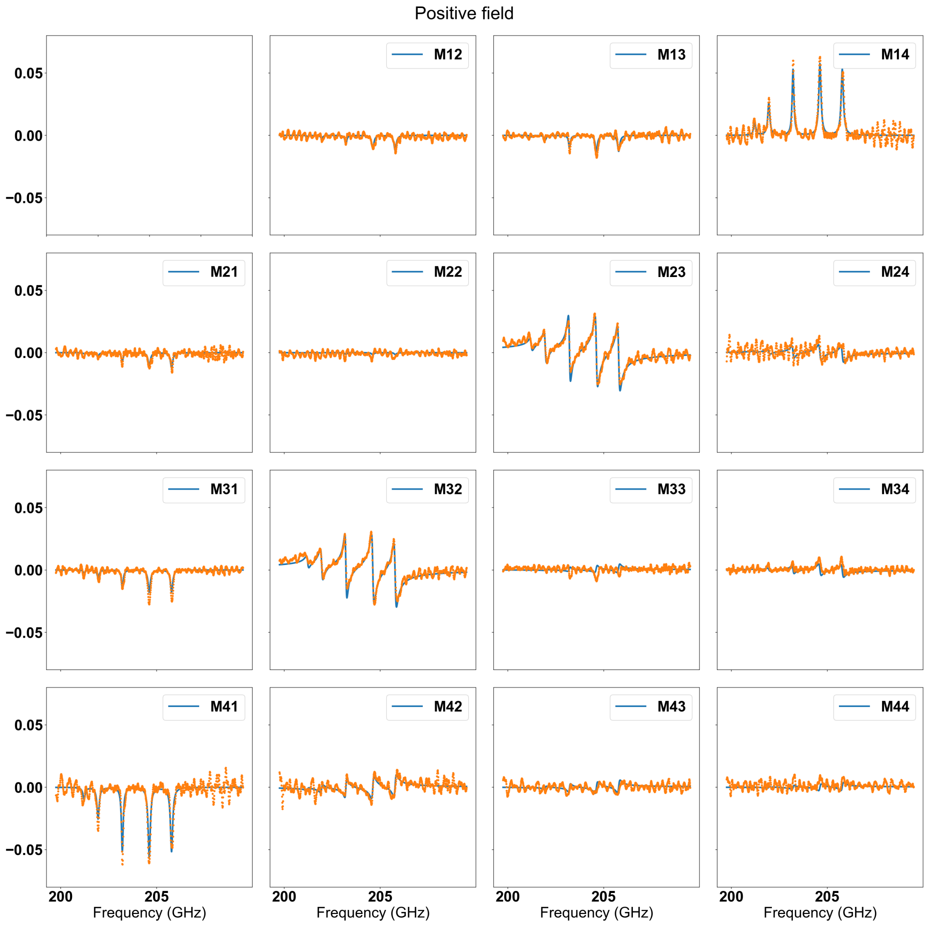


FIG. 1. Orange dots show experimental data gathered from terahertz magnetic resonance ellipsometry at 20 K. The data is the difference between a 0 T and a 7.23 T measurement. The blue solid line corresponds to the calculated best-match model as per the Bloch model derived in the main paper.

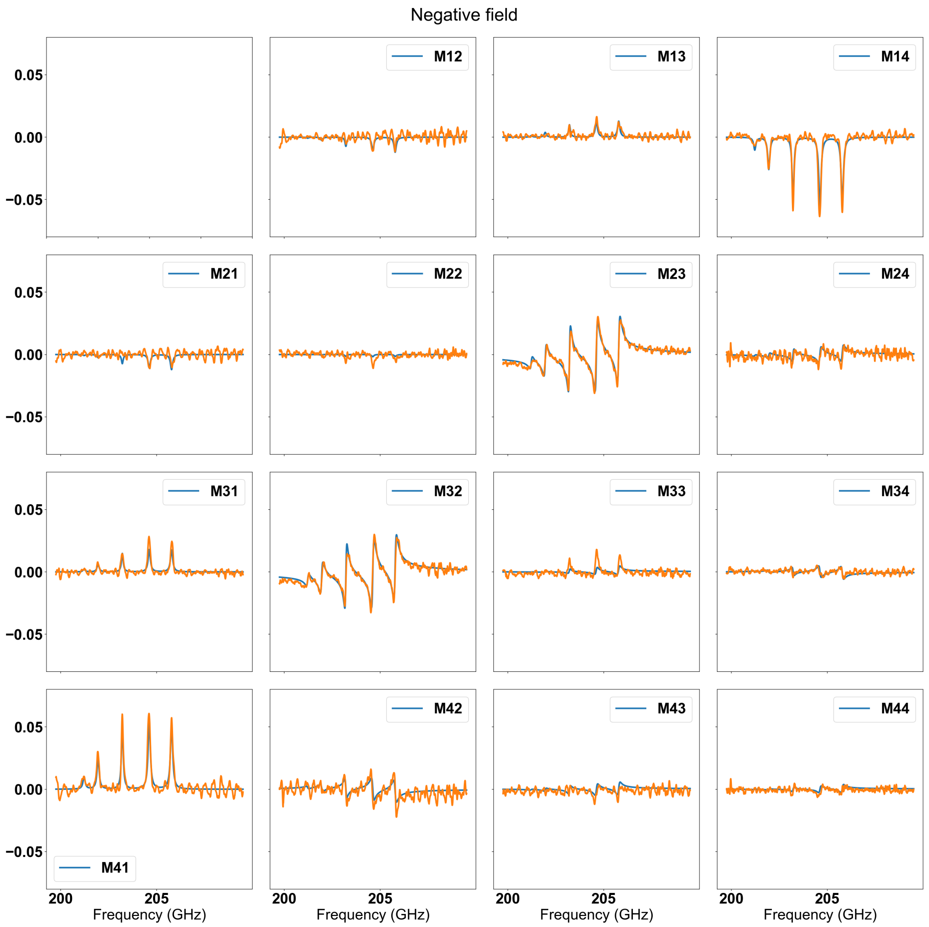


FIG. 2. Same as Fig. 1 but with a negative-valued magnetic field strength of -7.23 T.

---

* Electronic mail: viktor.rindert@ftf.lth.se
